# Supplementary material for: Attention-based Domain Adaptation for Single Stage Detectors
Source: arXiv:2106.07283 source file (2021-08-20)
Supplement: Supplementary file 1 [file supplementary.tex]

% !TEX root = ../top_sup.tex
% !TEX spellcheck = en-US

\section{Architecture Details}

The details of our detector's architecture are as follows.
\subsection{Backbone}
\textbf{SSD:} As mentioned in the main paper, we add an FPN~\cite{lin2017feature} to our VGG backbone. We use 7 scales corresponding to feature maps of size $64^2$, $32^2$, $16^2$, $8^2$, $4^2$, $2^2$, $1$ for our SSD architecture. We add a GroupNorm~\cite{wu2018group} layer after every convolutional layer. We set $D = C_s = 256$ for all pyramid levels, corresponding to the number of channel in the feature maps $F_s$.

\textbf{YOLOv5:} $D=C_s =128$, $256$, $512$ corresponds to the three YOLO feature levels with the backbone proposed in~\cite{glenn_jocher_2020_4154370}.

\subsection{Self Attention}
Figure~\ref{fig:attn_mod} depicts our self attention module design. Following~\cite{detr}, we add a feed forward network (FFN) and pass its output as an input to the detector heads. The FFN consists two fully-connected layers with $2048$ hidden units followed by $ReLU$ activation. Furthermore, we add a $Dropout$ layer with a factor of $0.1$, as in~\cite{detr}. We use LayerNorm~\cite{ba2016layer} to normalize the features. Finally, following~\cite{detr}, we set the number of heads for the multi-head attention layer to be $8$.
% !TEX root = ../top_sup.tex
% !TEX spellcheck = en-US
\begin{figure}[t]
\centering
\begin{tabular}{c}
\includegraphics[width=.45\linewidth]{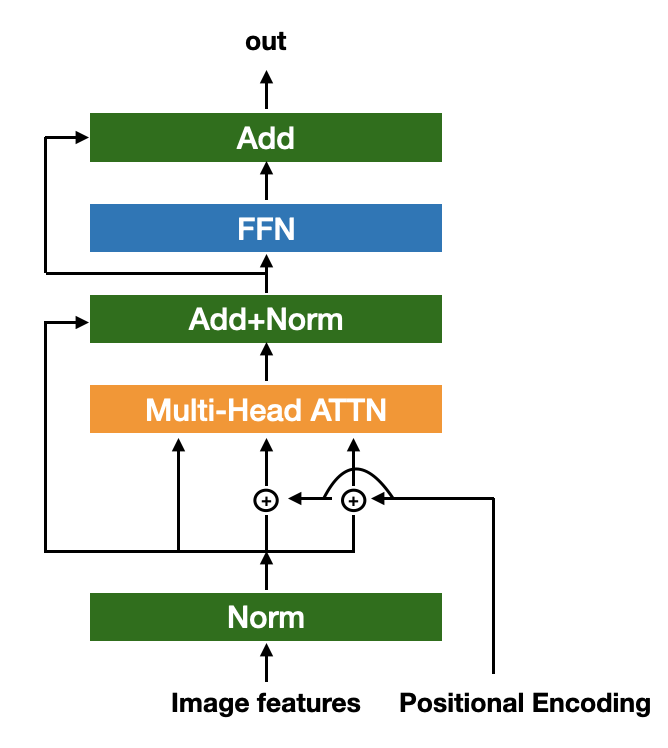}
\end{tabular}
  \caption{{\bf Self Attention Module}: Following~\cite{detr}, we use multihead attention followed by a feed forward network.} 

  \label{fig:attn_mod}
  \end{figure}

For SSD, we incorporate the attention module to the first three scales and use the third scale's attention map for remaining 4 scales using max-pooling to adapt the spatial resolution. This limits the increase in model complexity.
% and the scales with features map size $8^2$, $4^2$, $2^2$ and $1$, can resuse the attention from the lower scale. 
For YOLO, all three scales have an attention module.

\subsection{Discriminator}
We use blocks of $3\times 3$ convolution kernels with GroupNorm~\cite{wu2018group}, $ReLU$ activation and max-pooling with a stride of $2$. For a feature map of size $2^n\times2^n$, the discriminator at the corresponding scale contains $n$ blocks. These blocks are followed by a fully connected layer with $2$ hidden units.

\section{Training Details}
As discussed in the main paper, we define a factor $\gamma = \frac{2}{1+\exp(-\delta\cdot r)}-1$ to modulate the influence of attention on our feature maps. Here,
$r=\frac{current\,iteration'}{max\,iteration'}$ is computed from the moment the GRL is activated. Hence, $current\,iteration'$ = $current\,iteration - t_{grl}$  and $max\,iteration'$= $max\,iteration-t_{grl}$. $t_{grl}$ is the iteration at which the GRL begins the domain adaptation phase of training. 

\textbf{SSD:}
 We keep GRL activation iteration $t_{grl}=12k,12k,5k$ and $max\,iteration=30k,30k,50k$ for \textbf{S$\rightarrow$C}, \textbf{K$\rightarrow$C} and \textbf{C$\rightarrow$F}, respectively, reflecting the fact that \textbf{C$\rightarrow$F} has less training data. For \textbf{S$\rightarrow$C}, \textbf{K$\rightarrow$C}, we set the detector learning rate to 1e-3 for the first 10k iterations and then decay it by a  factor of 0.1. For \textbf{C$\rightarrow$F}, to avoid overfitting to the smaller source data, we set the learning rate to 5e-4  and decay it by 0.1 after 20k iterations. The discriminator learning rate is an order of magnitude smaller than the initial detector one and kept constant throughout training. This lets us train the attention layers faster than the discriminator for the initial iterations. Furthermore, the GRL coefficient is set to 0.005 for \textbf{S$\rightarrow$C} and \textbf{K$\rightarrow$C}, and to 0.5 for \textbf{C$\rightarrow$F} to compensate for the lower detector learning rate. We set $\delta$ to $5$. 

\textbf{YOLOv5:} We initially train without activating the GRL layer for 3 epochs in all cases and then set its coefficient to be 0.1. The base detector learning rate is set to be 0.1, and we train the model with $\delta$ set to 5. 
In these experiments, we set $t_{grl}=10$ epochs and $max\,epoch$=20,20,50 for {\bf S$\rightarrow$ C}, {\bf K$\rightarrow$ C} and {\bf C$\rightarrow$ F}, respectively. The initial learning rate is set to 0.001 for {\bf S$\rightarrow$ C} and 0.01 for {\bf K$\rightarrow$ C} and  {\bf C$\rightarrow$ F}. The GRL coefficient is 0.01 for {\bf S$\rightarrow$ C} and 0.1 for {\bf K$\rightarrow$ C} and  {\bf C$\rightarrow$ F}.

\section{Qualitative Results}
In Figures~\ref{fig:attenmapss2c}, \ref{fig:attenmapsc2f}, and~\ref{fig:attenmapsk2c}, we provide additional visual results obtained with our method applied to SSD.
% !TEX root = ../top_sup.tex
% !TEX spellcheck = en-US
\begin{figure*}[t]
\centering
\begin{tabular}{cc}
\includegraphics[width=.4\linewidth]{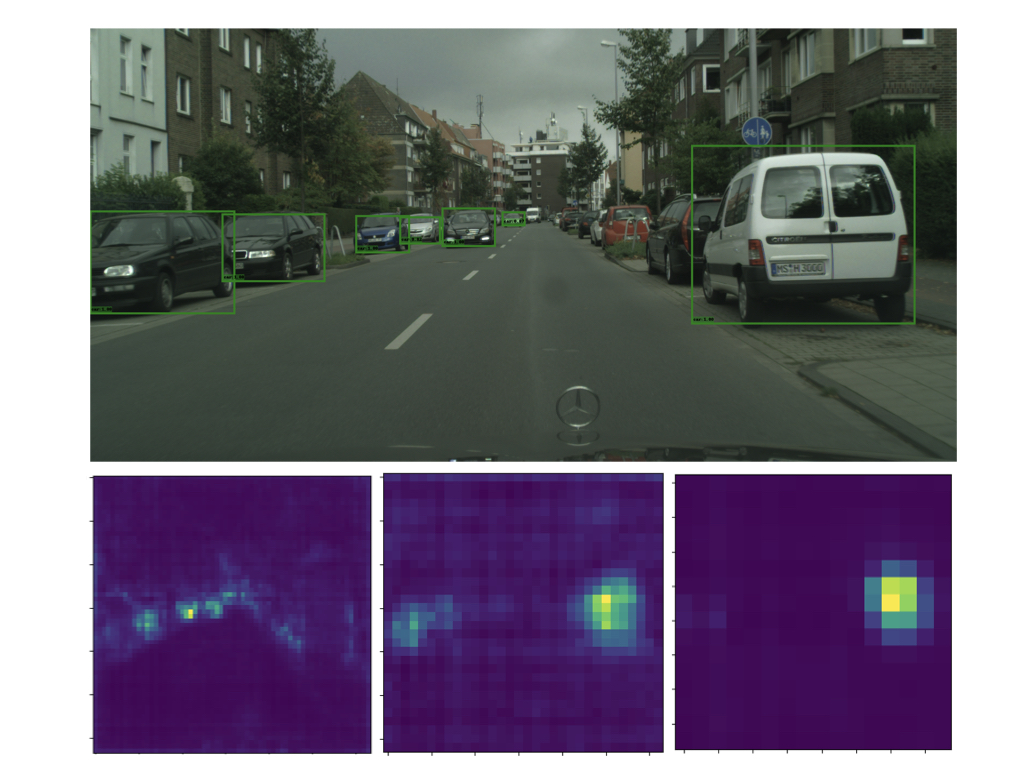}&
\includegraphics[width=.4\linewidth]{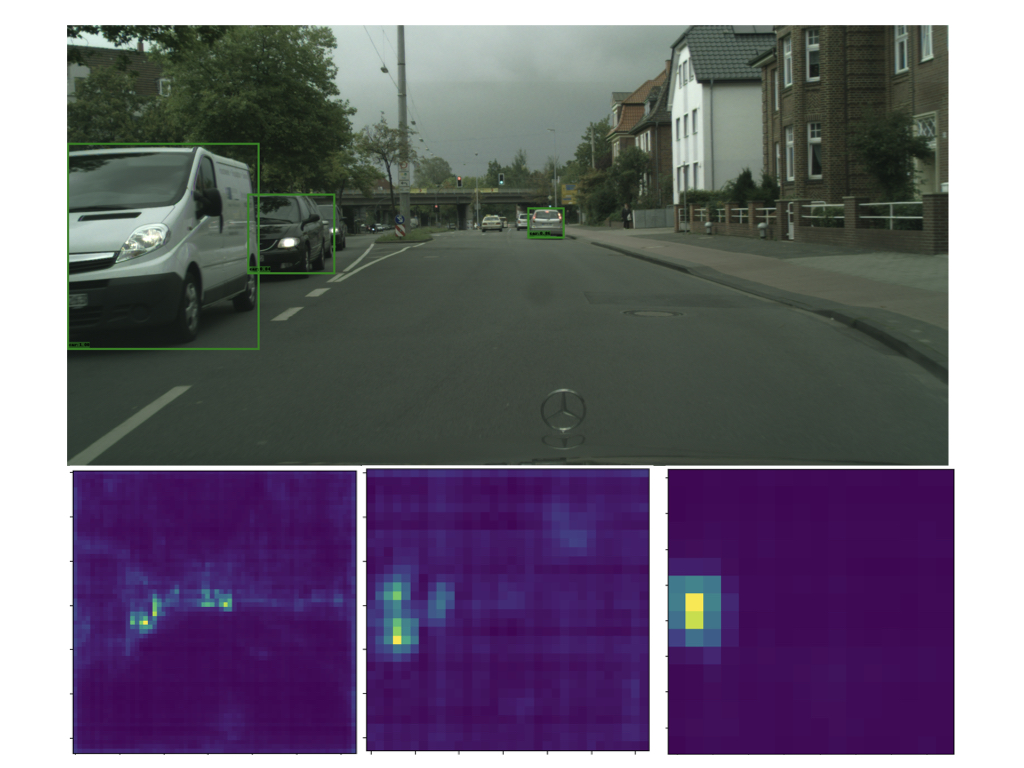}\\

\includegraphics[width=.4\linewidth]{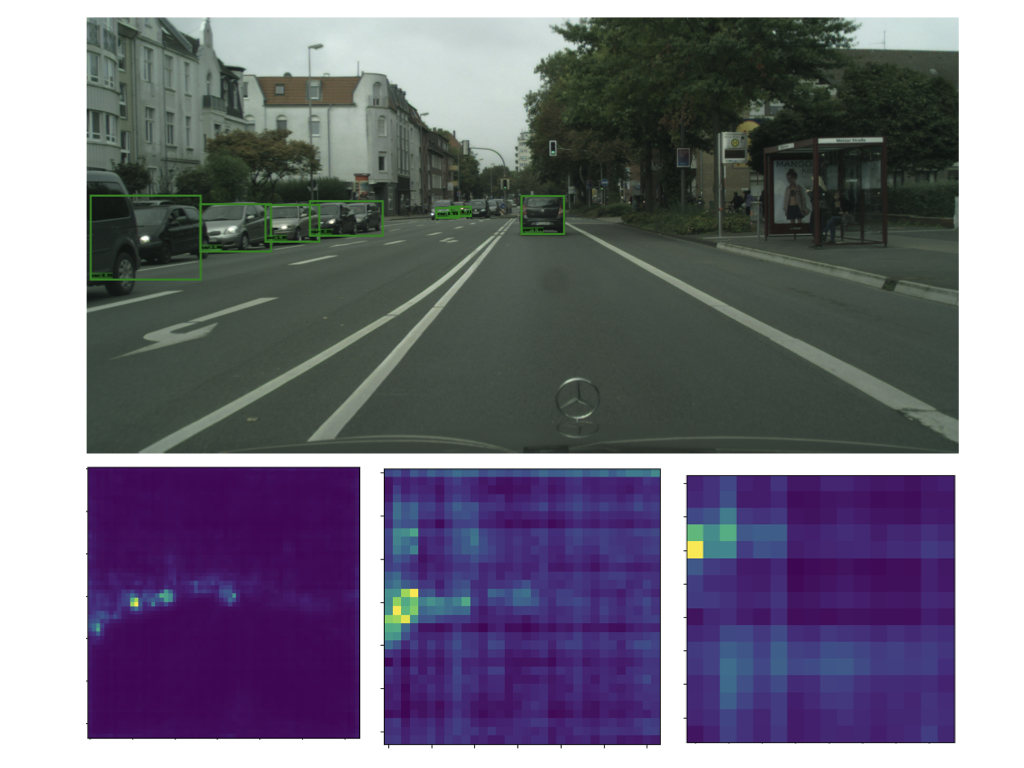}&
\includegraphics[width=.4\linewidth]{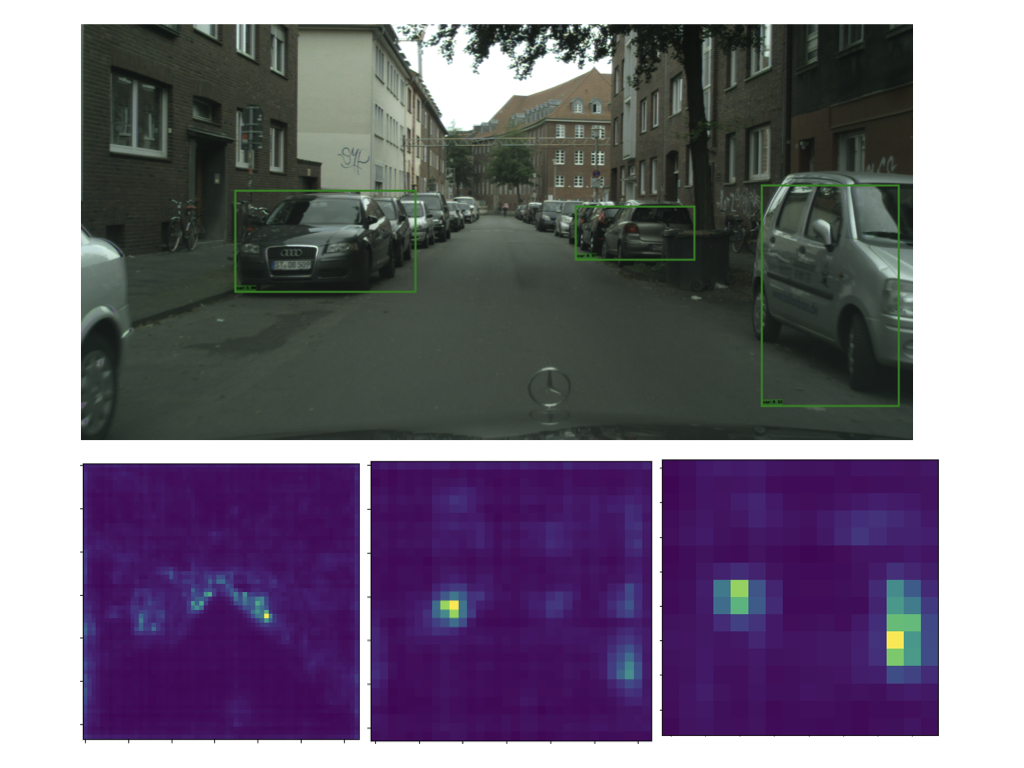}\\

\includegraphics[width=.4\linewidth]{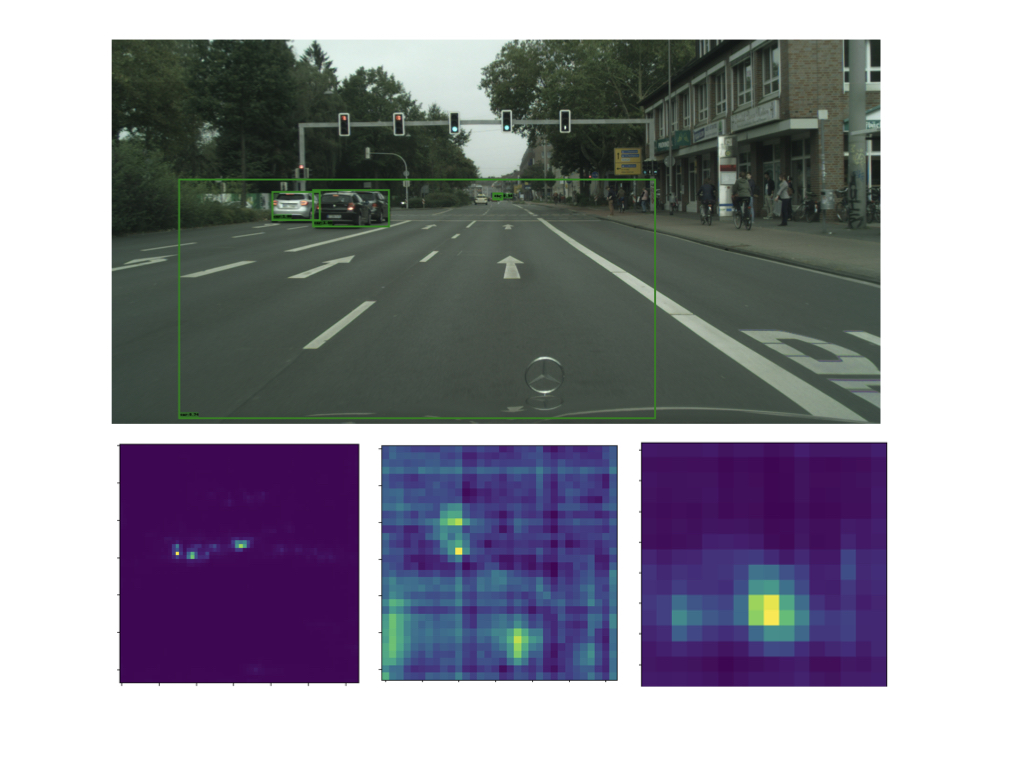}&
\includegraphics[width=.4\linewidth]{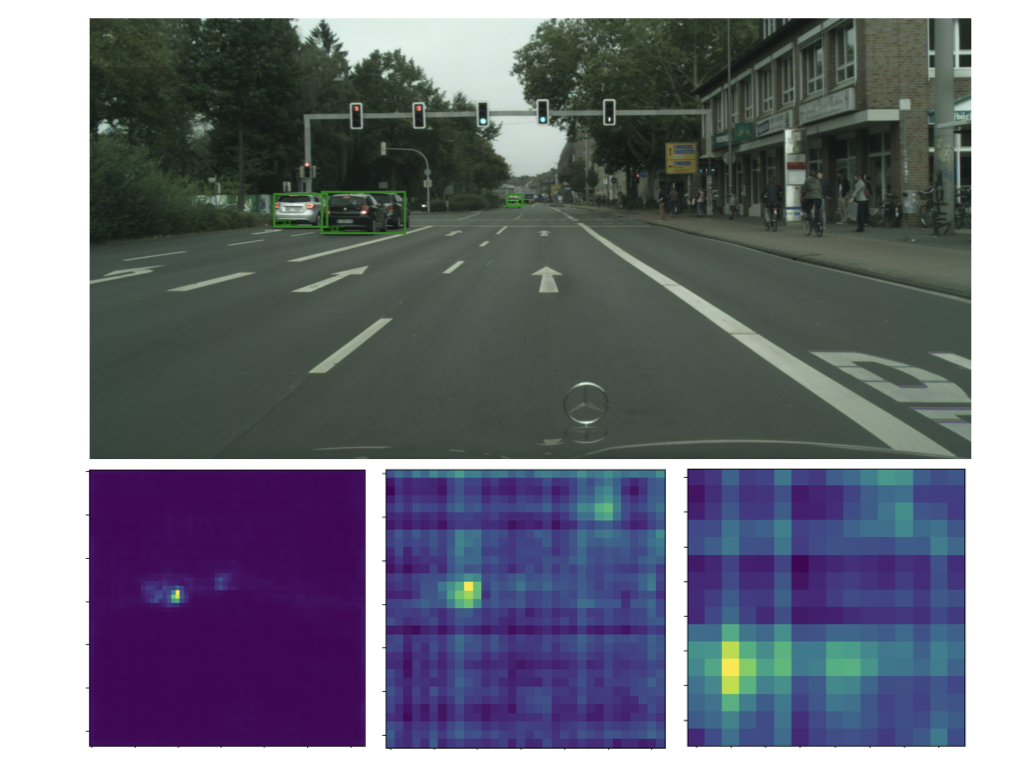}\\

\includegraphics[width=.4\linewidth]{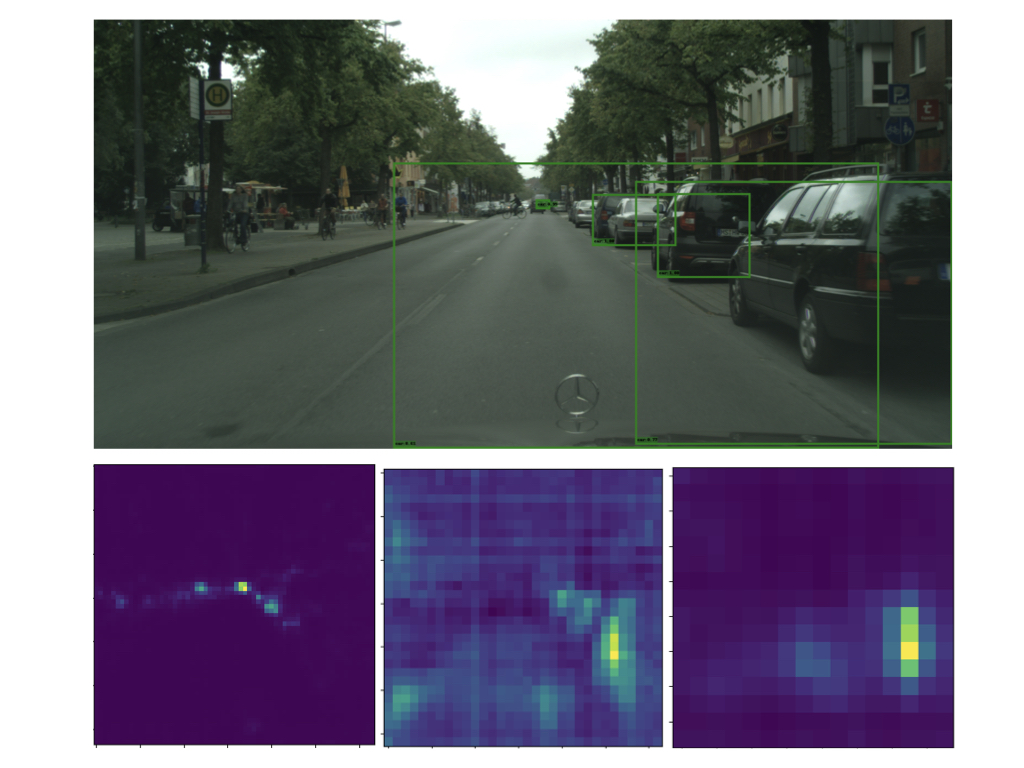}&
\includegraphics[width=.4\linewidth]{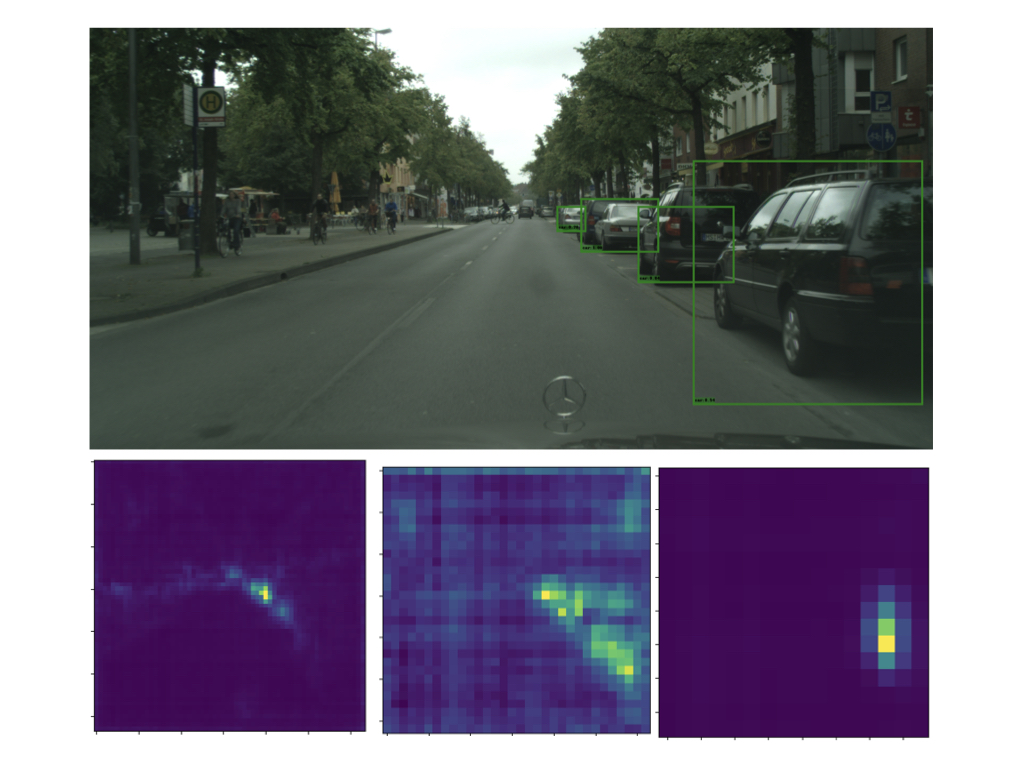}\\

\end{tabular}
\caption{{\bf Qualitative results on \textbf{S$\rightarrow$ C.} }We show targeted images with predicted detections, together with attention maps at different scales. All predictions are with confidence 50\% and above. \textbf{Bottom two rows:} We show the predictions and attention maps before(\textbf{left}) and after(\textbf{right}) adaptation. We can see we supress the false postives by learning better attention maps(middle). 
 }
\label{fig:attenmapss2c}
  \end{figure*}
% !TEX root = ../top_sup.tex
% !TEX spellcheck = en-US
\begin{figure*}[t]
\centering
\begin{tabular}{cc}
\includegraphics[width=.4\linewidth]{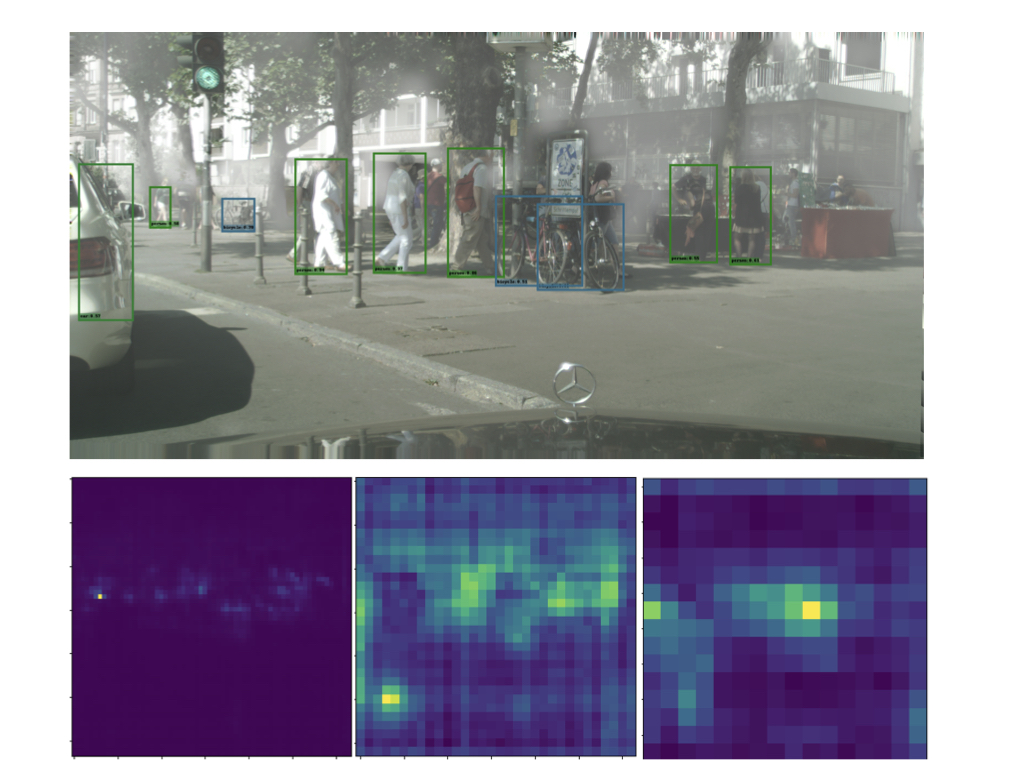}&
\includegraphics[width=.4\linewidth]{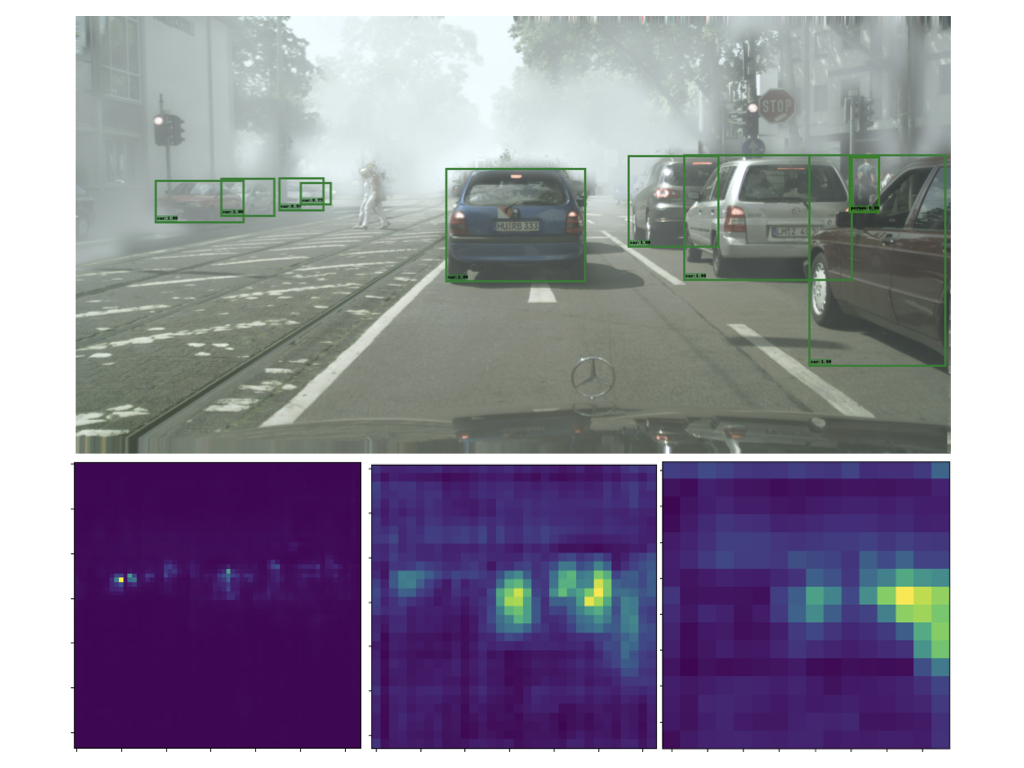}\\

\includegraphics[width=.4\linewidth]{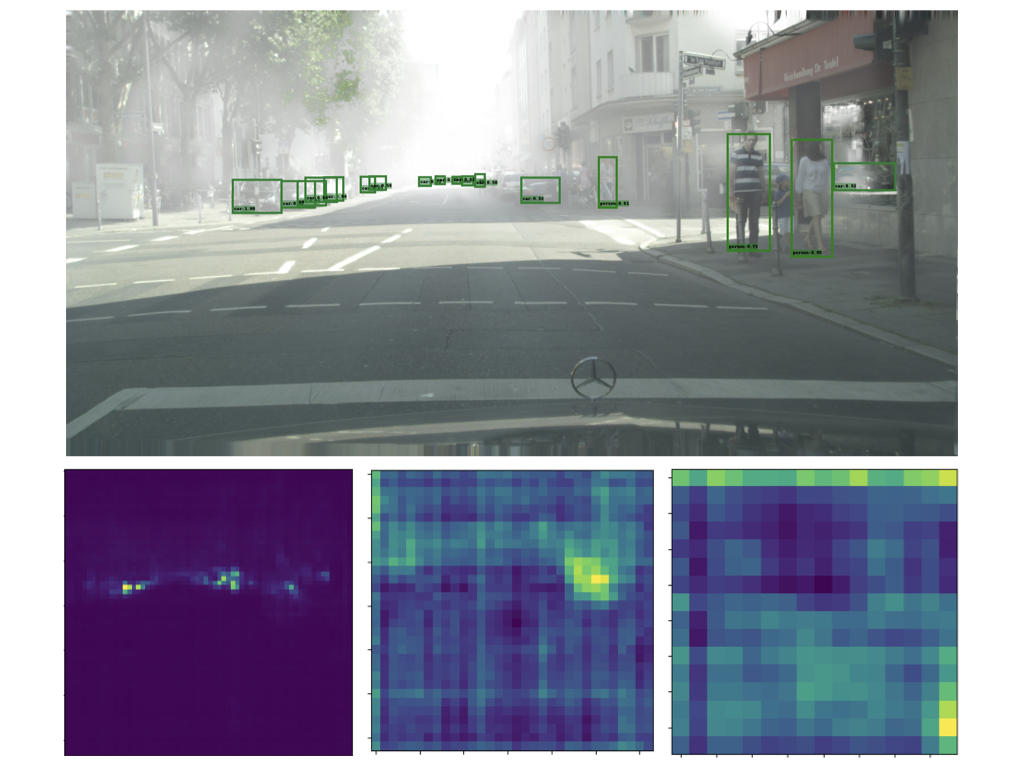}&
\includegraphics[width=.4\linewidth]{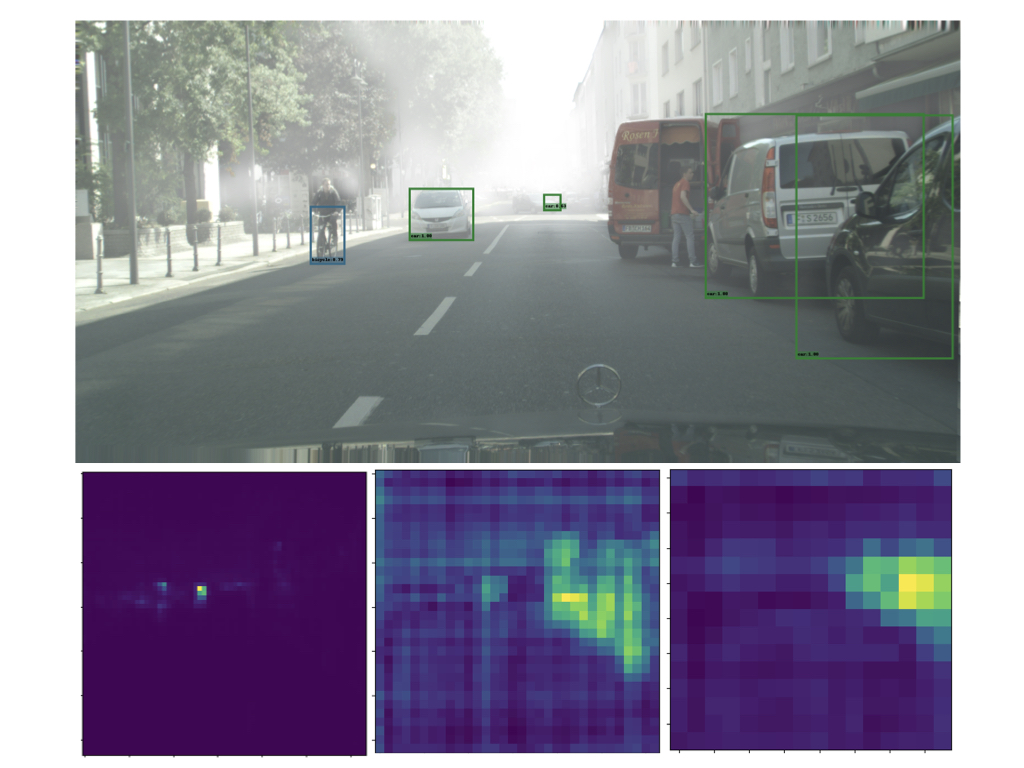}\\

\includegraphics[width=.4\linewidth]{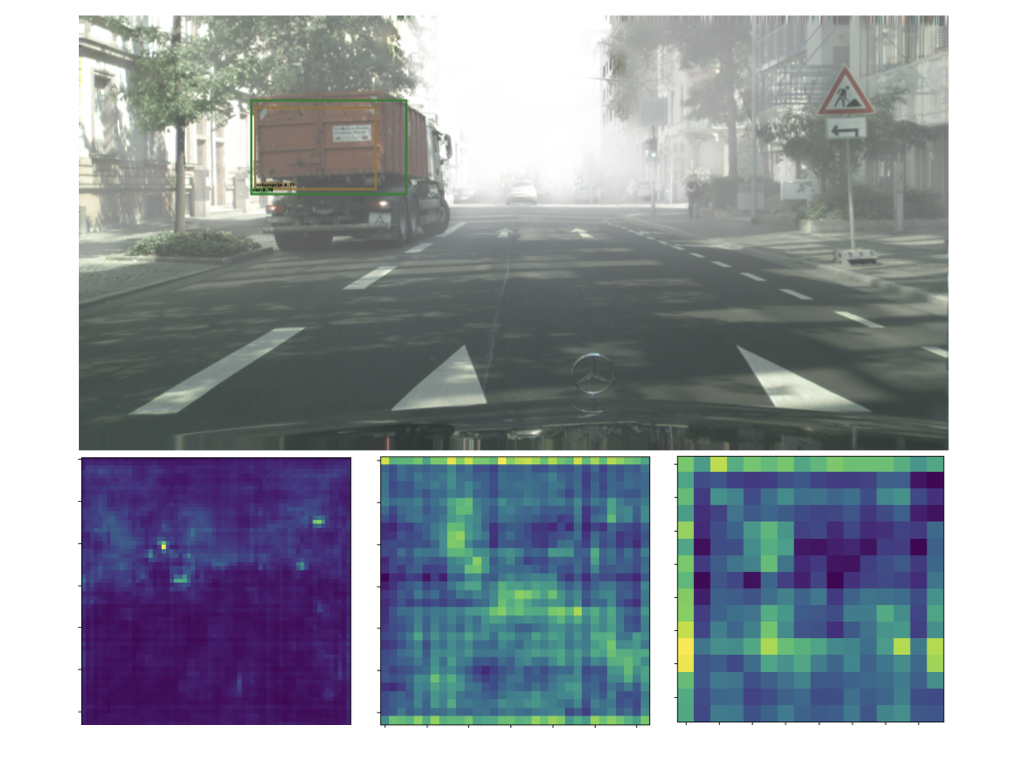}&
\includegraphics[width=.4\linewidth]{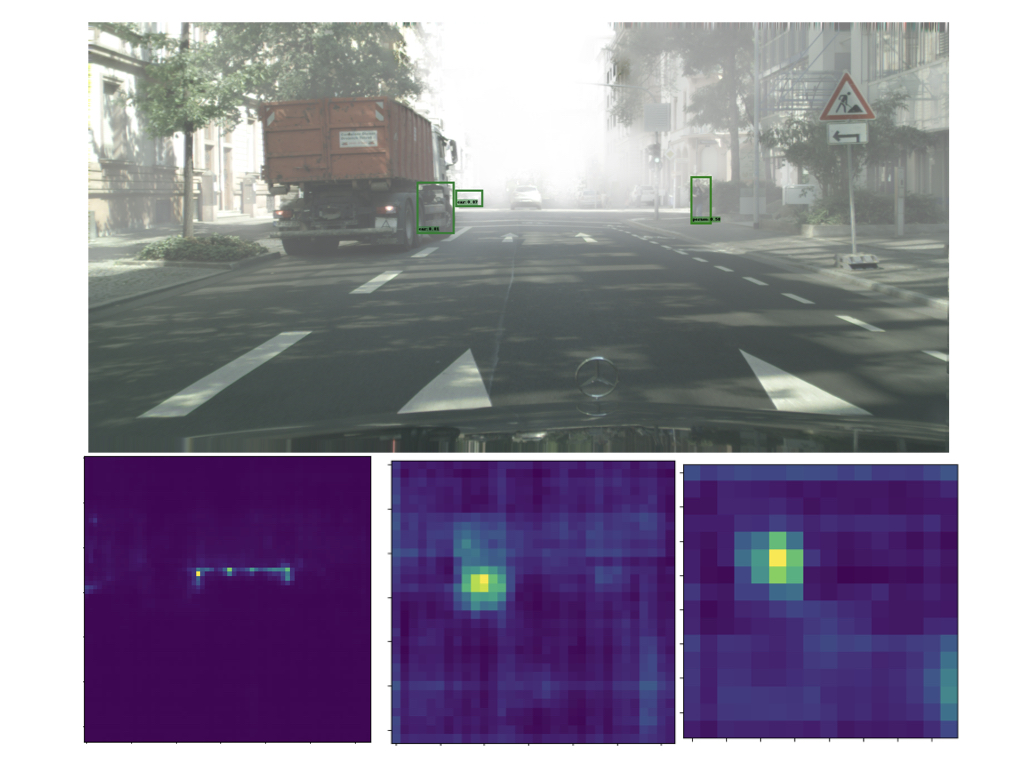}\\

\includegraphics[width=.4\linewidth]{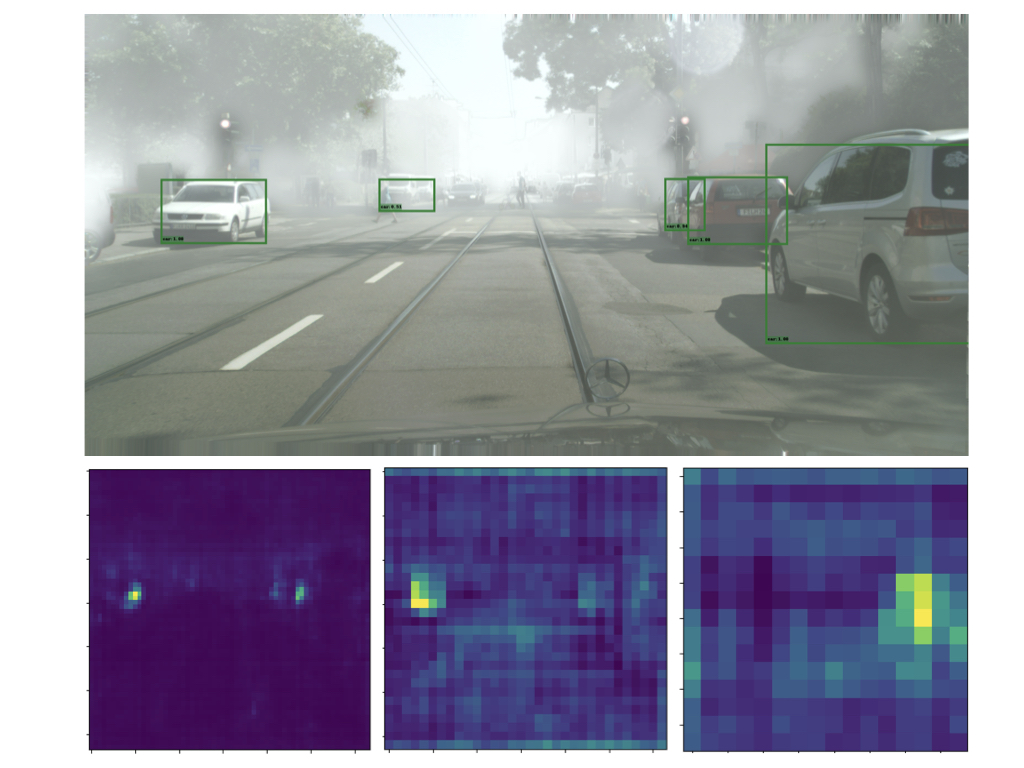}&
\includegraphics[width=.4\linewidth]{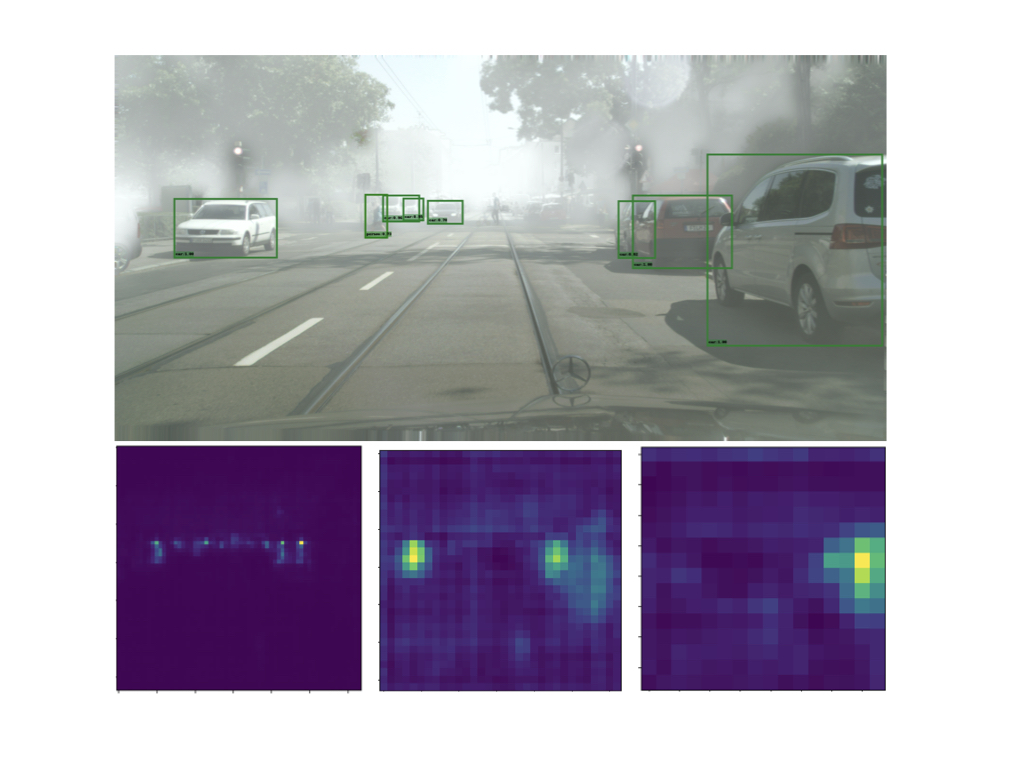}\\

\end{tabular}
\caption{{\bf Qualitative results on \textbf{C$\rightarrow$ F.} }We show targeted images with predicted detections, together with attention maps at different scales. Recall that here we consider multiple classes.All predictions are with confidence 50\% and above. \textbf{Bottom two rows:} We show the predictions and attention maps before(\textbf{left}) and after(\textbf{right}) adaptation. We are able to reduce the false positives and improve the detection on smaller objects in this case. 
 }
\label{fig:attenmapsc2f}
  \end{figure*}
% !TEX root = ../top_sup.tex
% !TEX spellcheck = en-US
\begin{figure*}[t]
\centering
\begin{tabular}{cc}
\includegraphics[width=.45\linewidth]{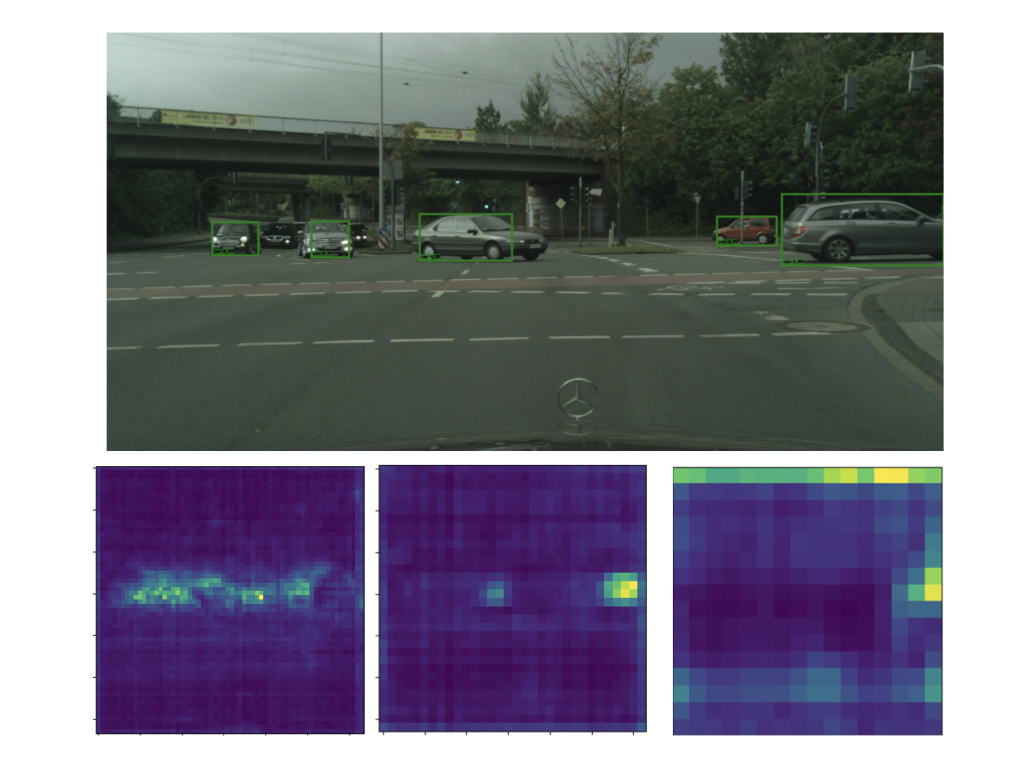}&
\includegraphics[width=.45\linewidth]{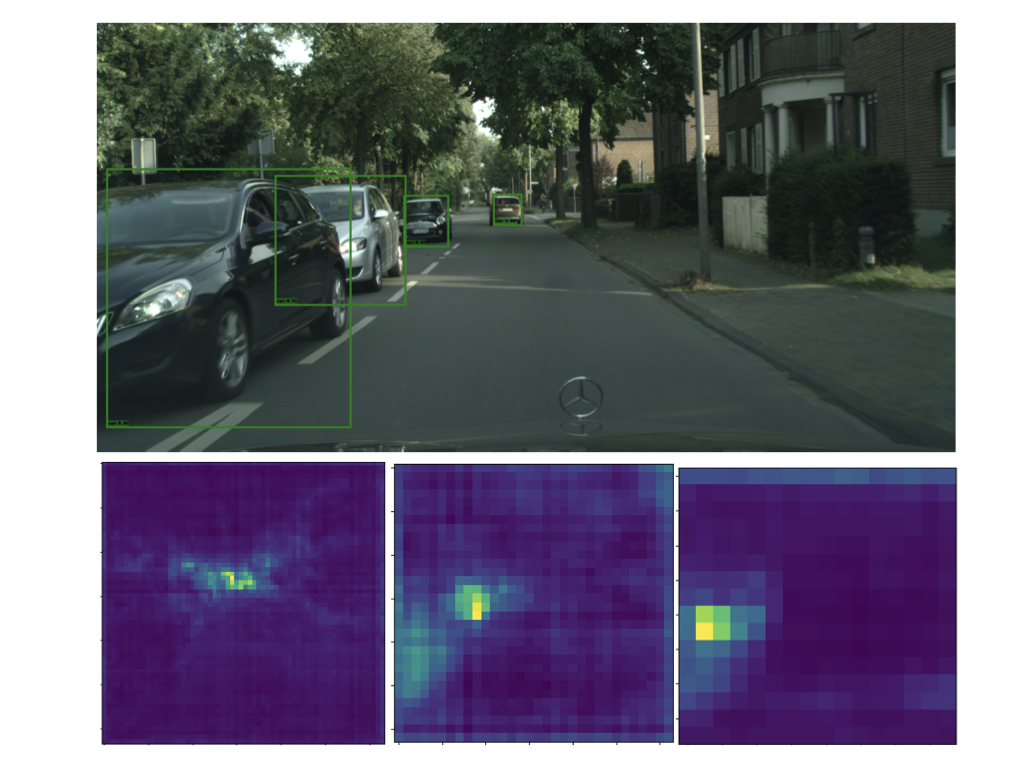}\\

\includegraphics[width=.45\linewidth]{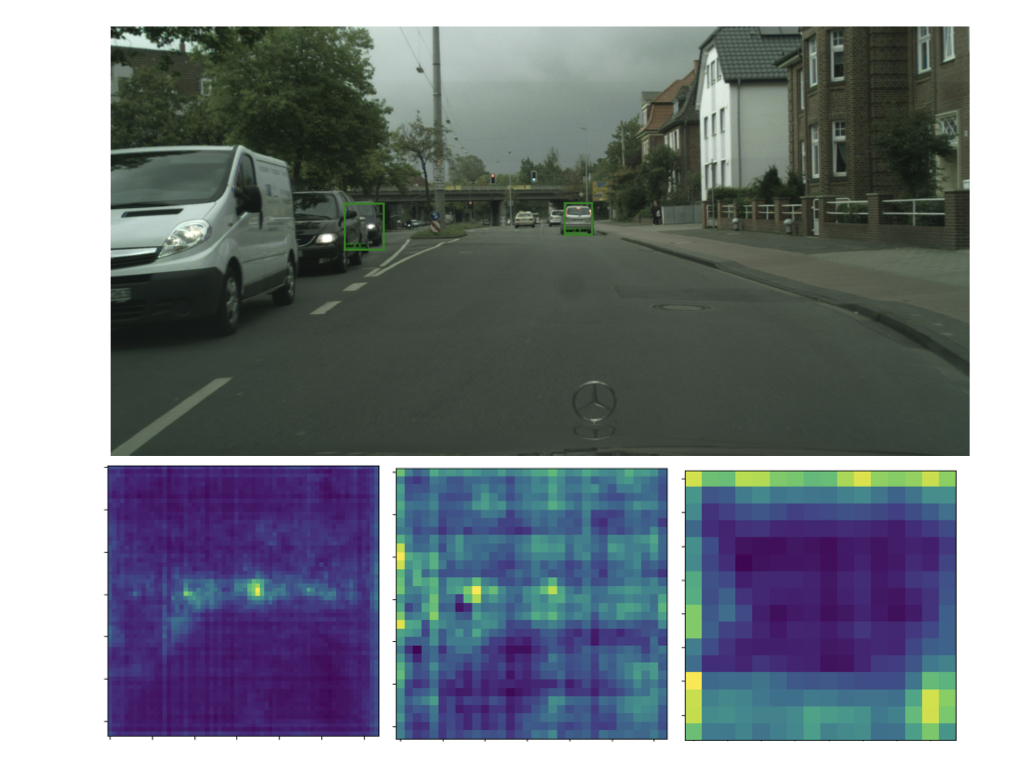}&
\includegraphics[width=.45\linewidth]{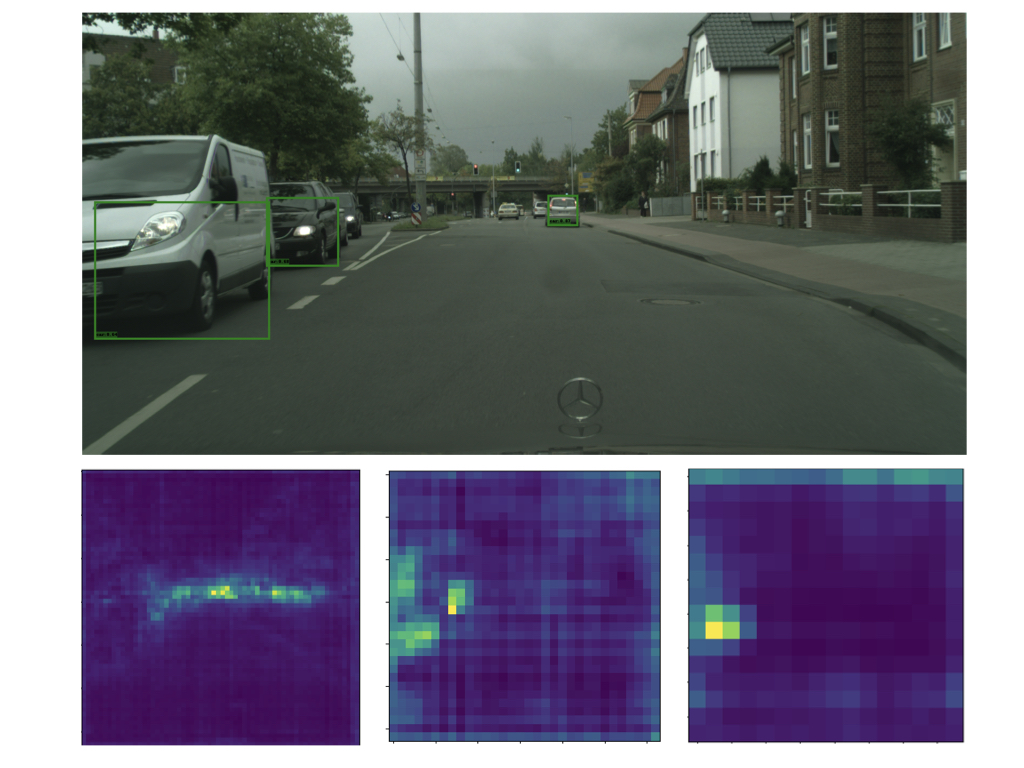}\\

\end{tabular}
\caption{{\bf Qualitative results on \textbf{K$\rightarrow$ C.} }We show targeted images with predicted detections, together with attention maps at different scales. All predictions are with confidence 50\% and above. \textbf{Bottom row:} We show the predictions and attention maps before(\textbf{left}) and after(\textbf{right}) adaptation. After adaptation, we see attention maps to be more focused on the foreground objects. 
 }
\label{fig:attenmapsk2c}
  \end{figure*}
