# Supplementary material for: Attention-based Domain Adaptation for Single Stage Detectors
Source: arXiv:2106.07283 source file (2021-08-20)
Supplement: Supplementary file 3 [file k2c_supp.tex]

% !TEX root = ../top_sup.tex
% !TEX spellcheck = en-US
\begin{figure*}[t]
\centering
\begin{tabular}{cc}
\includegraphics[width=.45\linewidth]{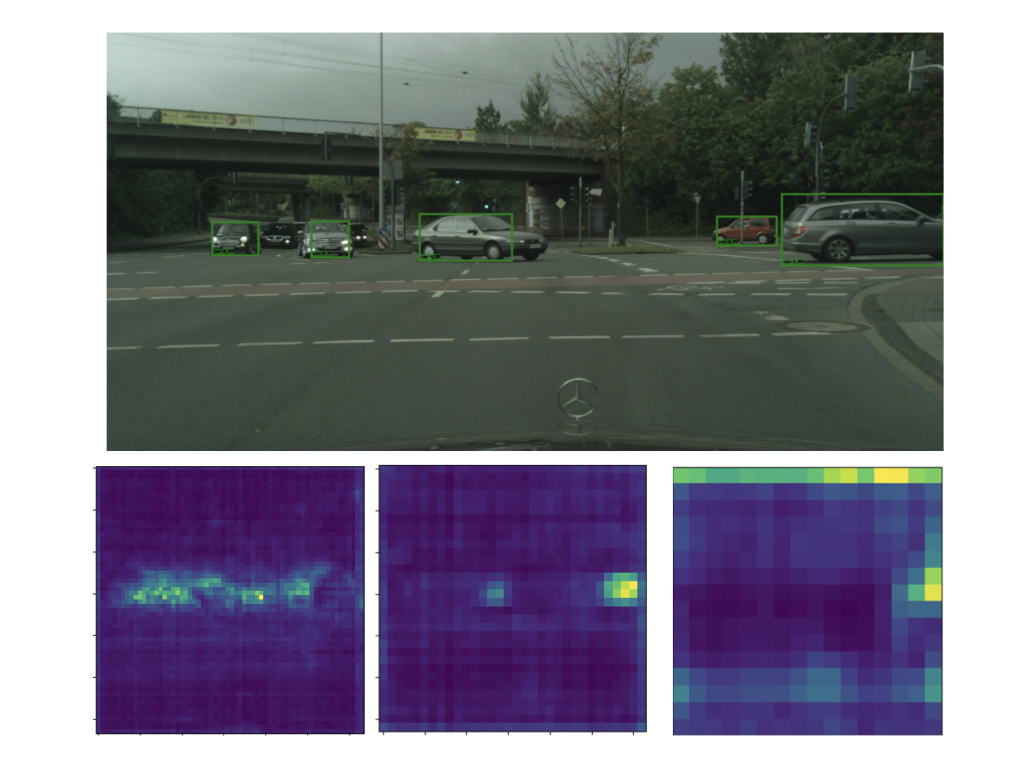}&
\includegraphics[width=.45\linewidth]{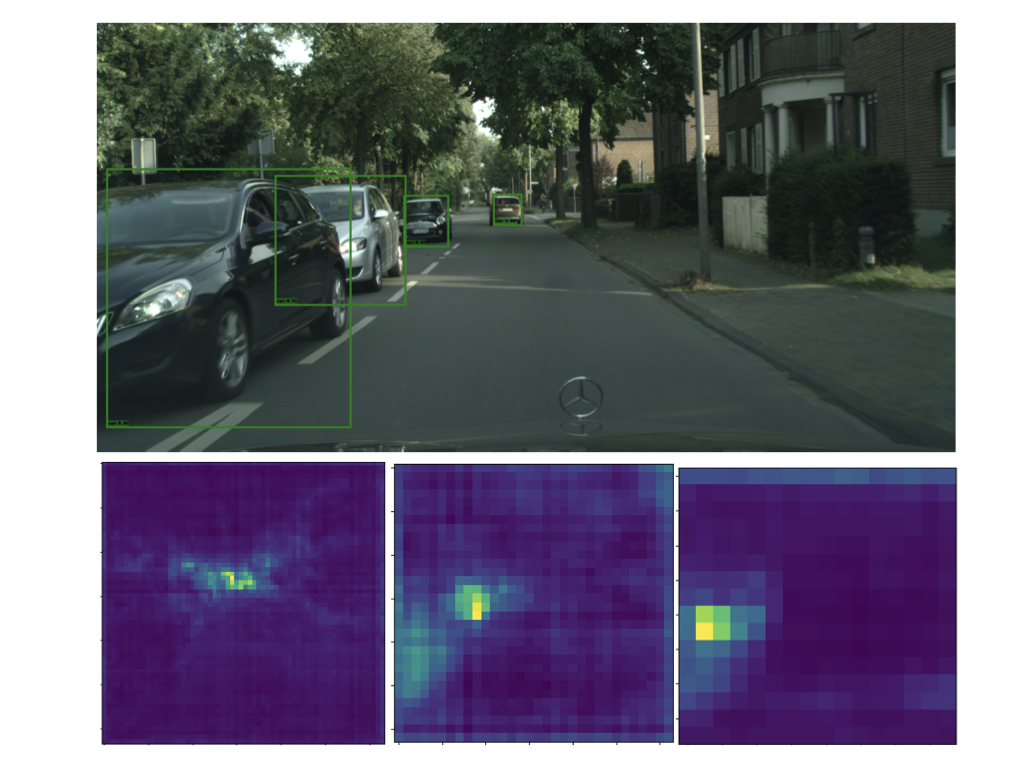}\\

\includegraphics[width=.45\linewidth]{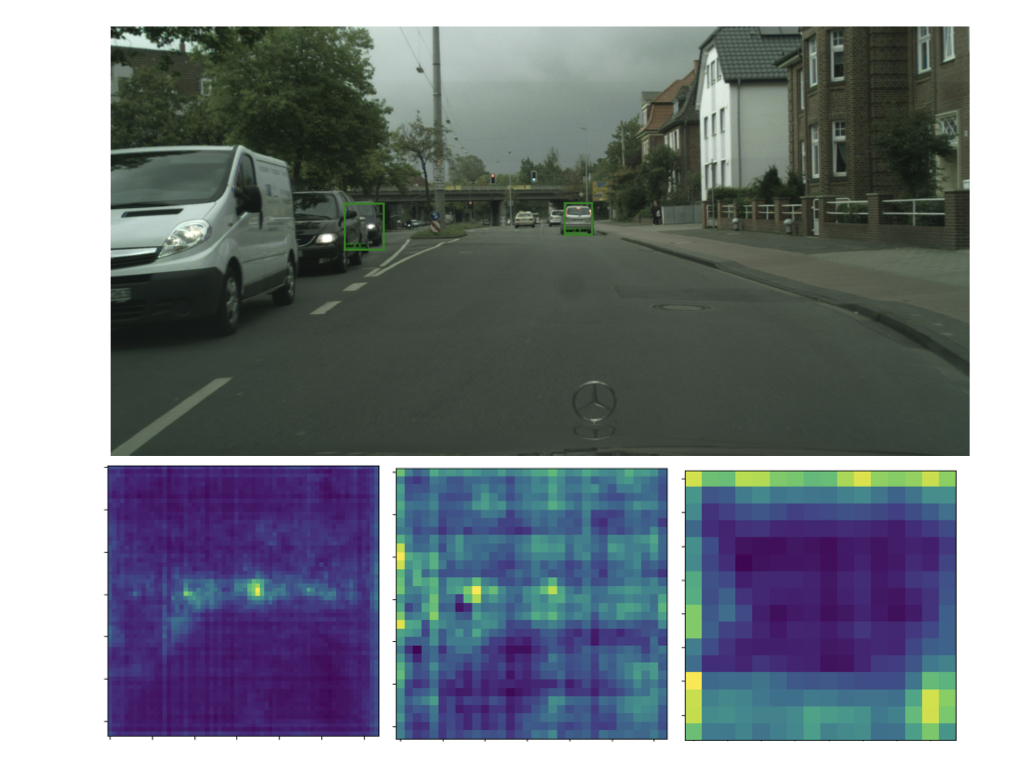}&
\includegraphics[width=.45\linewidth]{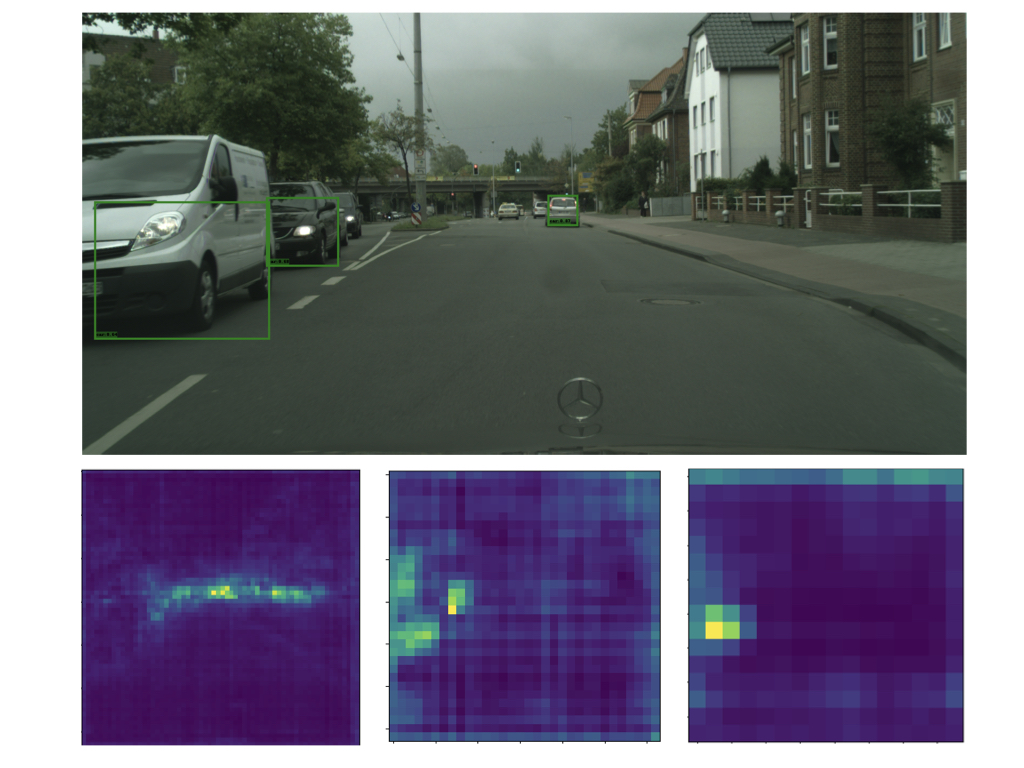}\\

\end{tabular}
\caption{{\bf Qualitative results on \textbf{K$\rightarrow$ C.} }We show targeted images with predicted detections, together with attention maps at different scales. All predictions are with confidence 50\% and above. \textbf{Bottom row:} We show the predictions and attention maps before(\textbf{left}) and after(\textbf{right}) adaptation. After adaptation, we see attention maps to be more focused on the foreground objects. 
 }
\label{fig:attenmapsk2c}
  \end{figure*}
