# Supplementary material for: Attention-based Domain Adaptation for Single Stage Detectors
Source: arXiv:2106.07283 source file (2021-08-20)
Supplement: Supplementary file 4 [file s2c_supp.tex]

% !TEX root = ../top_sup.tex
% !TEX spellcheck = en-US
\begin{figure*}[t]
\centering
\begin{tabular}{cc}
\includegraphics[width=.4\linewidth]{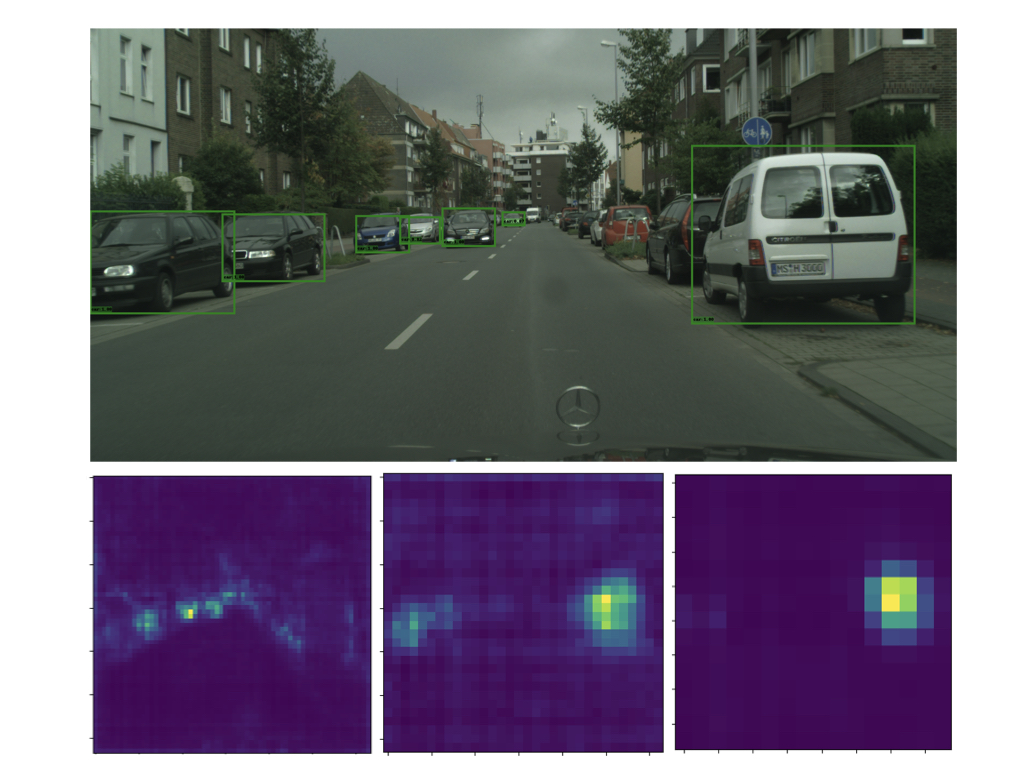}&
\includegraphics[width=.4\linewidth]{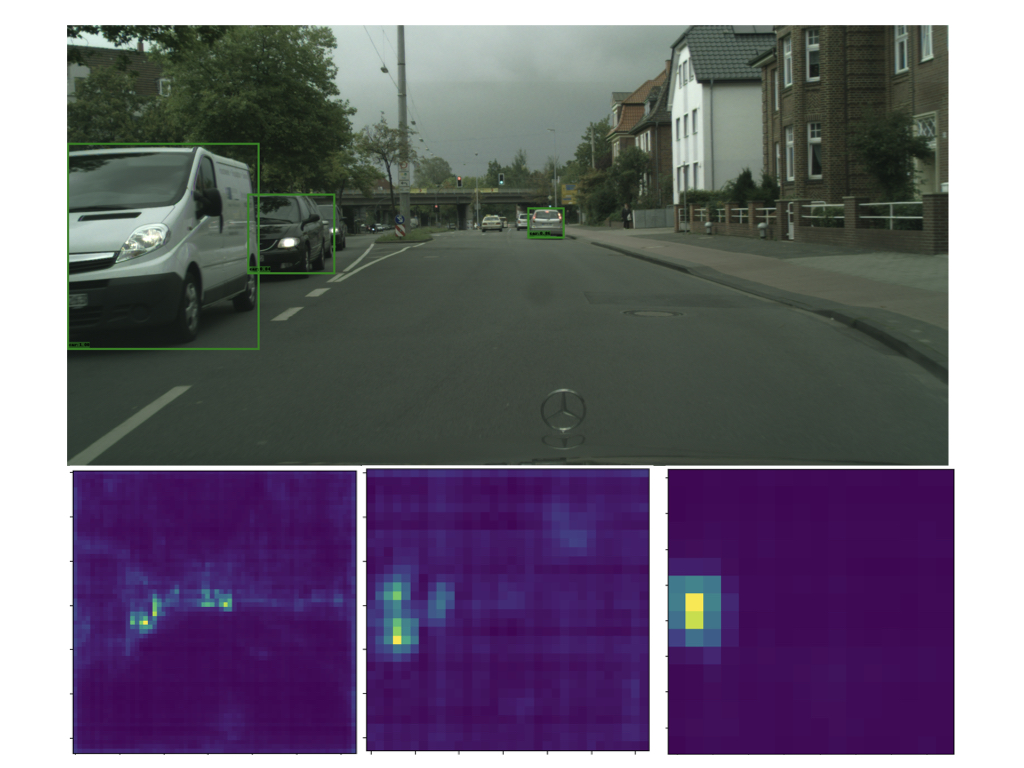}\\

\includegraphics[width=.4\linewidth]{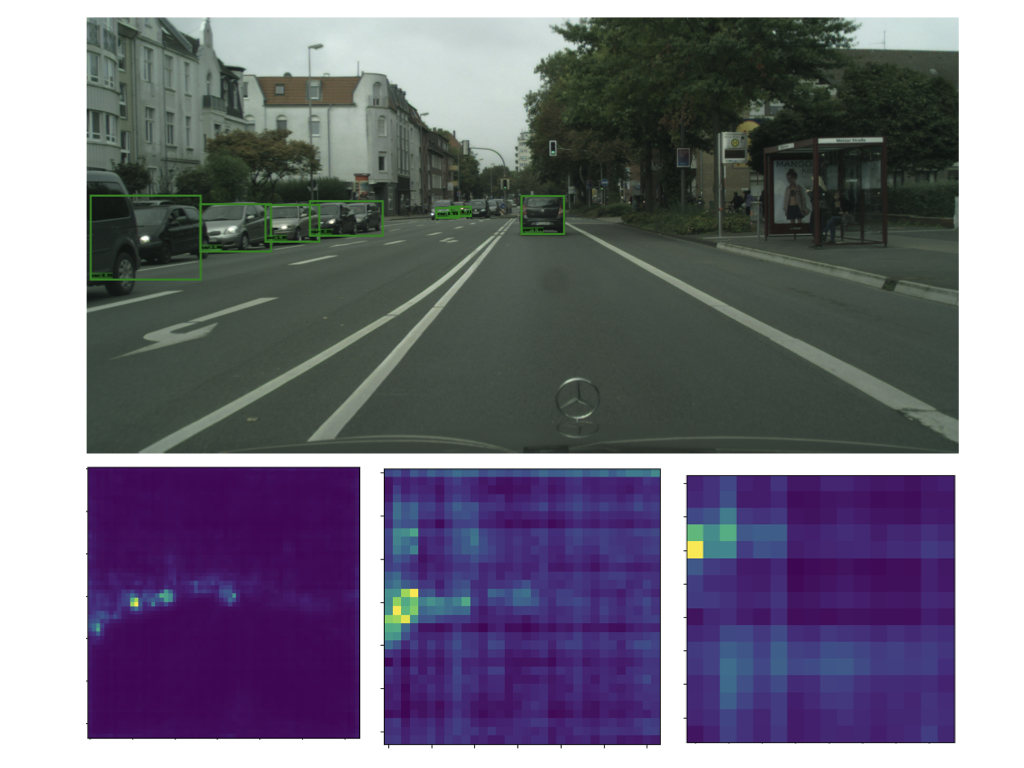}&
\includegraphics[width=.4\linewidth]{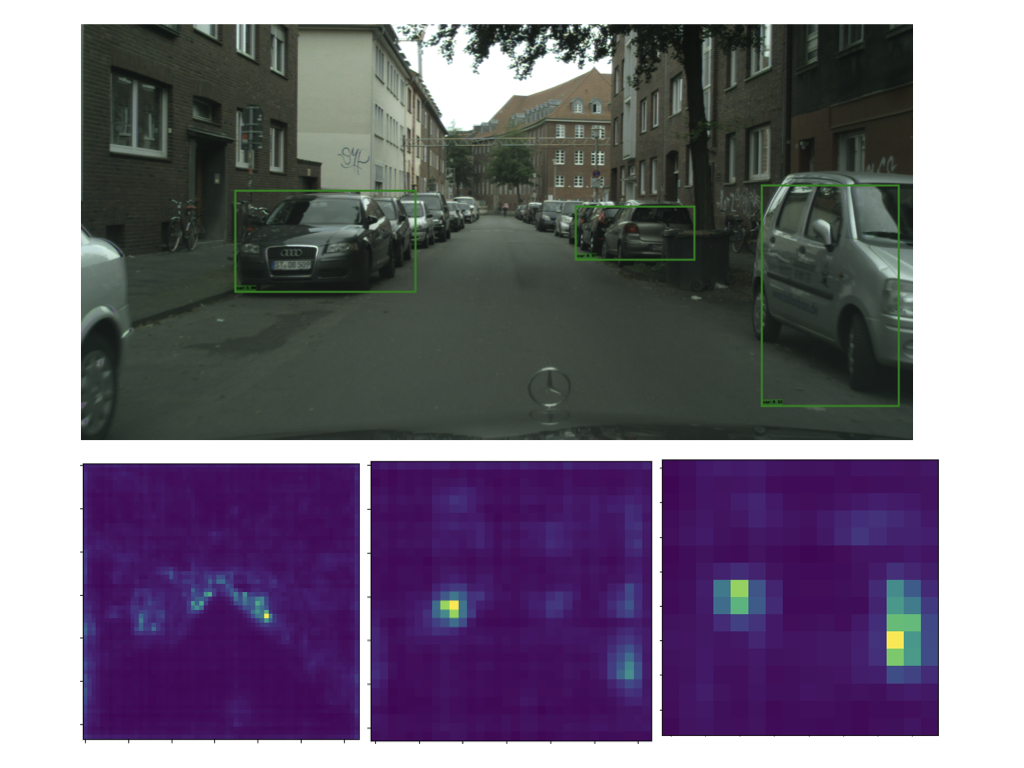}\\

\includegraphics[width=.4\linewidth]{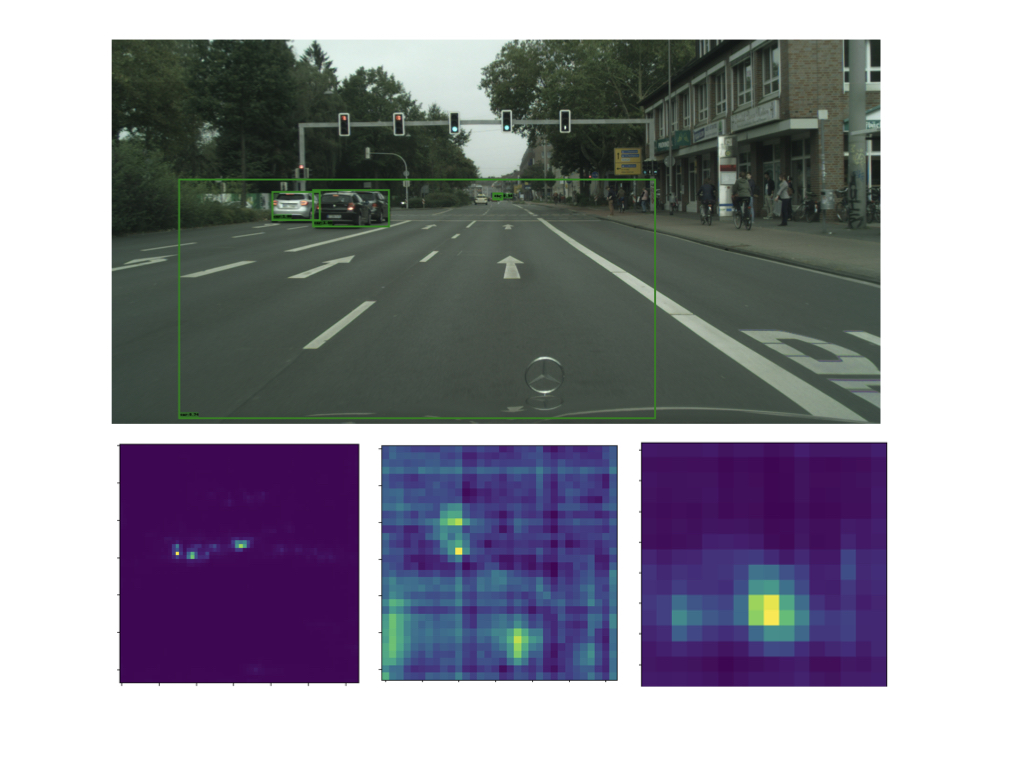}&
\includegraphics[width=.4\linewidth]{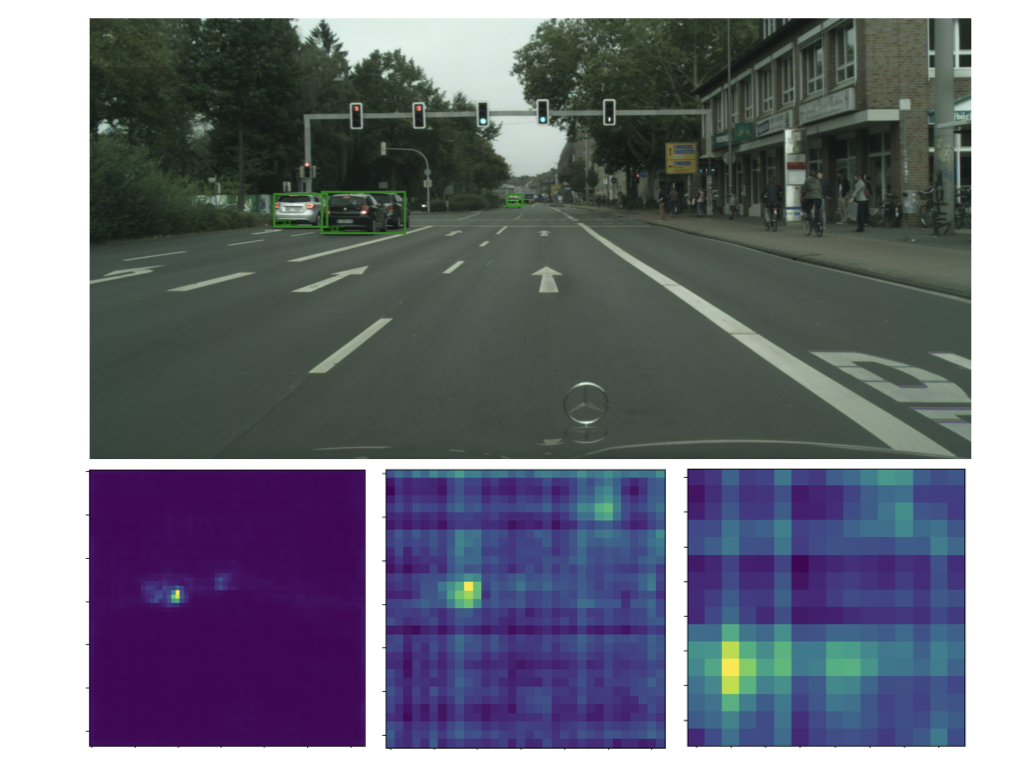}\\

\includegraphics[width=.4\linewidth]{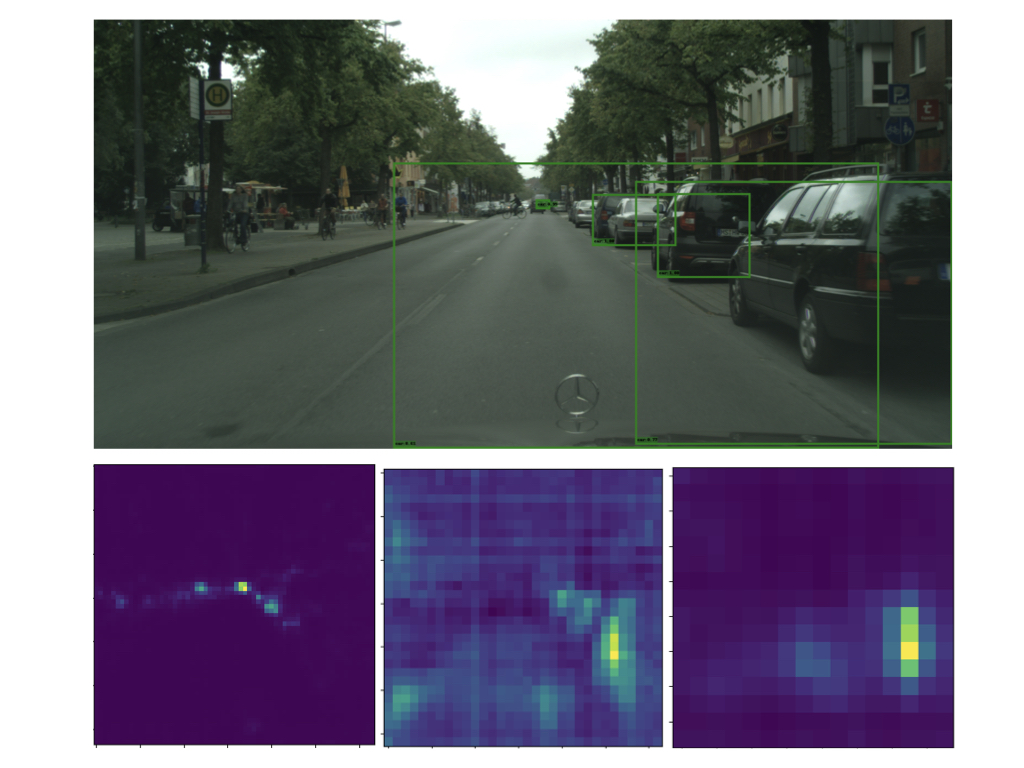}&
\includegraphics[width=.4\linewidth]{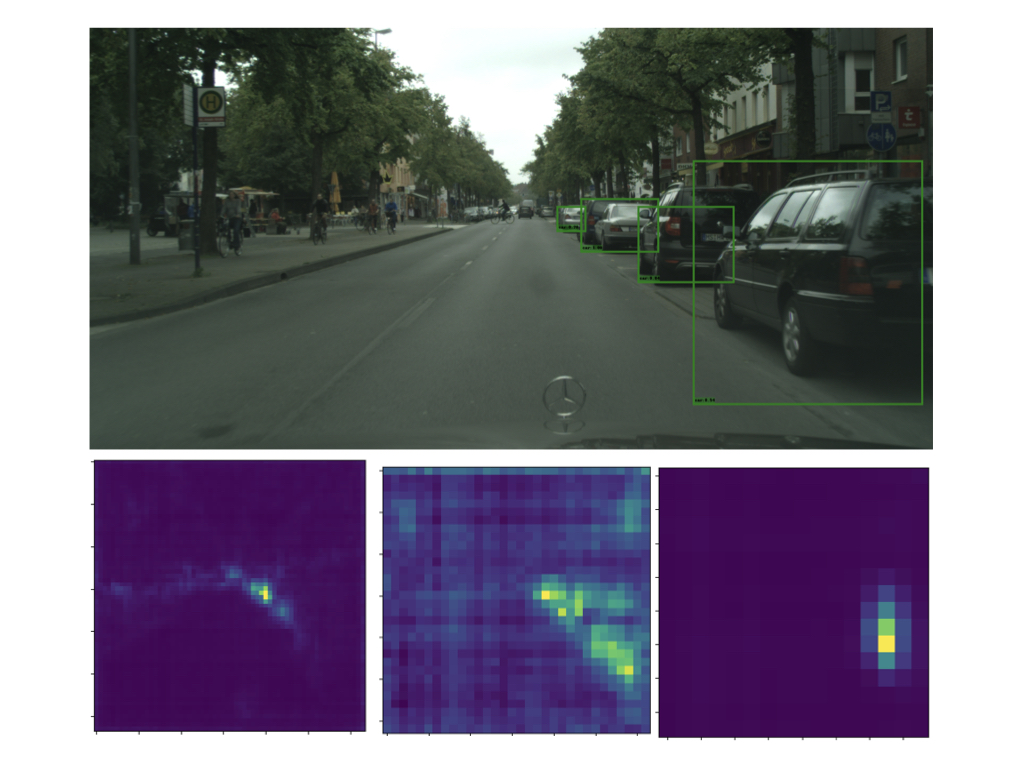}\\

\end{tabular}
\caption{{\bf Qualitative results on \textbf{S$\rightarrow$ C.} }We show targeted images with predicted detections, together with attention maps at different scales. All predictions are with confidence 50\% and above. \textbf{Bottom two rows:} We show the predictions and attention maps before(\textbf{left}) and after(\textbf{right}) adaptation. We can see we supress the false postives by learning better attention maps(middle). 
 }
\label{fig:attenmapss2c}
  \end{figure*}
